# Supplementary material for: cyTRON and cyTRON/JS: two Cytoscape-based applications for the inference of cancer evolution models
Source: arXiv:1705.03067 source file (2019-07-20)
Supplement: Supplementary file 1 [file supplementary.pdf]

# OncoScore: an R package to measure the oncogenic potential of genes

*Supplementary Information*

Daniele Ramazzotti\*    Luca De Sano\*    Roberta Spinelli  
Rocco Piazza    Carlo Gambacorti Passerini

OncoScore is a tool to measure the association of genes to cancer based on citation frequency in biomedical literature. The score is evaluated from PubMed literature by dynamically updatable web queries.

## 1 Installation

The *OncoScore* R package is available on *Bioconductor* at <https://bioconductor.org/packages/release/bioc/html/OncoScore.html> and can be installed as follows.

```
## try http:// if https:// URLs are not supported
source("https://bioconductor.org/biocLite.R")
biocLite("OncoScore")
```

The package is also available on *Github* at <https://github.com/danro9685/OncoScore>. It is possible to install both the master (stable) and development versions of the R package by using the R library *devtools*.

```
library(devtools)
install_github("danro9685/OncoScore", ref = 'master')
library(OncoScore)

library(devtools)
install_github("danro9685/OncoScore", ref = 'development')
library(OncoScore)
```

## 2 Examples

The OncoScore analysis consists of two parts. One can estimate a score to assess the oncogenic potential of a set of genes, given the literature knowledge, at the time of the analysis, or one can study the trend of such score over time.

---

\*Equal contributors.

We next present the two analysis and we conclude with showing the capabilities of the tool to visualize the results. First we load the library.

```
library(OncoScore)
```

## 2.1 OncoScore analysis

The query that we show next retrieves from PubMed the citations, at the time of the query, for a list of genes in cancer related and in all the documents.

```
query = perform.query(c("ASXL1", "IDH1", "IDH2", "SETBP1", "TET2"))
```

```
### Starting the queries for the selected genes.
```

```
### Performing queries for cancer literature
```

```
Number of papers found in PubMed for ASXL1 was: 309
Number of papers found in PubMed for IDH1 was: 1450
Number of papers found in PubMed for IDH2 was: 557
Number of papers found in PubMed for SETBP1 was: 69
Number of papers found in PubMed for TET2 was: 560
```

```
### Performing queries for all the literature
```

```
Number of papers found in PubMed for ASXL1 was: 350
Number of papers found in PubMed for IDH1 was: 1581
Number of papers found in PubMed for IDH2 was: 648
Number of papers found in PubMed for SETBP1 was: 89
Number of papers found in PubMed for TET2 was: 717
```

OncoScore also provides a function to retrieve the names of the genes in a given portion of a chromosome that can be exploited if we are dealing, e.g., with copy number alterations hitting regions rather than specific genes.

```
> chr13 = get.genes.from.biomart(chromosome=13,start=54700000,end=72800000)
> head(chr13)
```

```
[1] "LINC00374" "RNA5SP30" "RNU7-87P" "HNF4GP1" "RN7SL375P" "BORA"
```

Furthermore, one can also automatically perform the OncoScore analysis on chromosomal regions as follows:

```
> result = compute.oncoscore.from.region(10, 100000, 500000)
```

```
### Performing query on BioMart
```

```
### Performing web query on: RNA5SP297 RNA5SP298 RN7SL754P ZMYND11 DIP2C
```

```
### Starting the queries for the selected genes.
```

```
### Performing queries for cancer literature
```

```

Number of papers found in PubMed for RNA5SP297 was: -1
Number of papers found in PubMed for RNA5SP298 was: -1
Number of papers found in PubMed for RN7SL754P was: -1
Number of papers found in PubMed for ZMYND11 was: 27
Number of papers found in PubMed for DIP2C was: 1

### Performing queries for all the literature
Number of papers found in PubMed for RNA5SP297 was: -1
Number of papers found in PubMed for RNA5SP298 was: -1
Number of papers found in PubMed for RN7SL754P was: -1
Number of papers found in PubMed for ZMYND11 was: 45
Number of papers found in PubMed for DIP2C was: 3

### Processing data
### Computing frequencies scores
### Estimating oncogenes
### Results:
RNA5SP297 -> 0
RNA5SP298 -> 0
RN7SL754P -> 0
ZMYND11 -> 49.07473
DIP2C -> 12.30234

```

We now compute a score for each of the genes, to estimate their oncogenic potential.

```
> result = compute.oncoscore(query)
```

```

### Processing data
### Computing frequencies scores
### Estimating oncogenes
### Results:
ASXL1 -> 77.8392
IDH1 -> 83.08351
IDH2 -> 76.75356
SETBP1 -> 65.556
TET2 -> 69.86954

```

## 2.2 OncoScore timeline analysis

The query that we show next retrieves from PubMed the citations, at specified time points, for a list of genes in cancer related and in all the documents.

```
> query.timepoints = perform.query.timeseries(c("ASXL1", "IDH1", "IDH2",
"SETBP1", "TET2"), c("2012/03/01", "2013/03/01", "2014/03/01",
"2015/03/01", "2016/03/01"))
```

```

### Starting the queries for the selected genes.
### Querying PubMed for timepoint 2012/03/01
### Performing queries for cancer literature
Number of papers found in PubMed for ASXL1 was: 83
Number of papers found in PubMed for IDH1 was: 408
Number of papers found in PubMed for IDH2 was: 172
Number of papers found in PubMed for SETBP1 was: 5
Number of papers found in PubMed for TET2 was: 169
### Performing queries for all the literature
Number of papers found in PubMed for ASXL1 was: 91
Number of papers found in PubMed for IDH1 was: 488
Number of papers found in PubMed for IDH2 was: 234
Number of papers found in PubMed for SETBP1 was: 10
Number of papers found in PubMed for TET2 was: 196
### Querying PubMed for timepoint 2013/03/01
### Performing queries for cancer literature
Number of papers found in PubMed for ASXL1 was: 132
Number of papers found in PubMed for IDH1 was: 662
Number of papers found in PubMed for IDH2 was: 267
Number of papers found in PubMed for SETBP1 was: 11
Number of papers found in PubMed for TET2 was: 254
### Performing queries for all the literature
Number of papers found in PubMed for ASXL1 was: 149
Number of papers found in PubMed for IDH1 was: 753
Number of papers found in PubMed for IDH2 was: 336
Number of papers found in PubMed for SETBP1 was: 18
Number of papers found in PubMed for TET2 was: 302
### Querying PubMed for timepoint 2014/03/01
### Performing queries for cancer literature
Number of papers found in PubMed for ASXL1 was: 185
Number of papers found in PubMed for IDH1 was: 903
Number of papers found in PubMed for IDH2 was: 364
Number of papers found in PubMed for SETBP1 was: 29
Number of papers found in PubMed for TET2 was: 342
### Performing queries for all the literature
Number of papers found in PubMed for ASXL1 was: 208
Number of papers found in PubMed for IDH1 was: 1002
Number of papers found in PubMed for IDH2 was: 439
Number of papers found in PubMed for SETBP1 was: 36
Number of papers found in PubMed for TET2 was: 430
### Querying PubMed for timepoint 2015/03/01
### Performing queries for cancer literature
Number of papers found in PubMed for ASXL1 was: 250
Number of papers found in PubMed for IDH1 was: 1188
Number of papers found in PubMed for IDH2 was: 467
Number of papers found in PubMed for SETBP1 was: 49

```

```

Number of papers found in PubMed for TET2 was: 452
### Performing queries for all the literature
Number of papers found in PubMed for ASXL1 was: 283
Number of papers found in PubMed for IDH1 was: 1300
Number of papers found in PubMed for IDH2 was: 550
Number of papers found in PubMed for SETBP1 was: 64
Number of papers found in PubMed for TET2 was: 576
### Querying PubMed for timepoint 2016/03/01
### Performing queries for cancer literature
Number of papers found in PubMed for ASXL1 was: 309
Number of papers found in PubMed for IDH1 was: 1446
Number of papers found in PubMed for IDH2 was: 557
Number of papers found in PubMed for SETBP1 was: 69
Number of papers found in PubMed for TET2 was: 558
### Performing queries for all the literature
Number of papers found in PubMed for ASXL1 was: 350
Number of papers found in PubMed for IDH1 was: 1576
Number of papers found in PubMed for IDH2 was: 648
Number of papers found in PubMed for SETBP1 was: 89
Number of papers found in PubMed for TET2 was: 715

```

We now compute a score for each of the genes, to estimate their oncogenic potential at specified time points.

```

> result.timeseries = compute.oncoscore.timeseries(query.timepoints)

### Computing oncoscore for timepoint 2012/03/01
### Processing data
### Computing frequencies scores
### Estimating oncogenes
### Results:
      ASXL1 -> 77.19348
      IDH1  -> 74.24489
      IDH2  -> 64.1649
      SETBP1 -> 34.9485
      TET2  -> 74.90108
### Computing oncoscore for timepoint 2013/03/01
### Processing data
### Computing frequencies scores
### Estimating oncogenes
### Results:
      ASXL1 -> 76.31902
      IDH1  -> 78.71551
      IDH2  -> 69.99559
      SETBP1 -> 46.4559
      TET2  -> 73.89695

```

```

### Computing oncoscore for timepoint 2014/03/01
### Processing data
### Computing frequencies scores
### Estimating oncogenes
### Results:
      ASXL1 -> 77.39202
      IDH1  -> 81.07946
      IDH2  -> 73.46995
      SETBP1 -> 64.97398
      TET2  -> 70.44331
### Computing oncoscore for timepoint 2015/03/01
### Processing data
### Computing frequencies scores
### Estimating oncogenes
### Results:
      ASXL1 -> 77.49295
      IDH1  -> 82.55032
      IDH2  -> 75.58179
      SETBP1 -> 63.80208
      TET2  -> 69.91466
### Computing oncoscore for timepoint 2016/03/01
### Processing data
### Computing frequencies scores
### Estimating oncogenes
### Results:
      ASXL1 -> 77.8392
      IDH1  -> 83.11346
      IDH2  -> 76.75356
      SETBP1 -> 65.556
      TET2  -> 69.81125

```

## 2.3 Visualization of the results

We next plot the scores measuring the oncogenetic potential of the considered genes as a barplot (see Figure 1).

```
> plot.oncoscore(result, col = 'darkblue')
```

We finally plot the trend of the scores over the considered times as absolute and values and as relative variations (see Figures 2, 3, 4).

```

> plot.oncoscore.timeseries(result.timeseries)

> plot.oncoscore.timeseries(result.timeseries,
      incremental = TRUE,
      ylab='absolute variation')

```

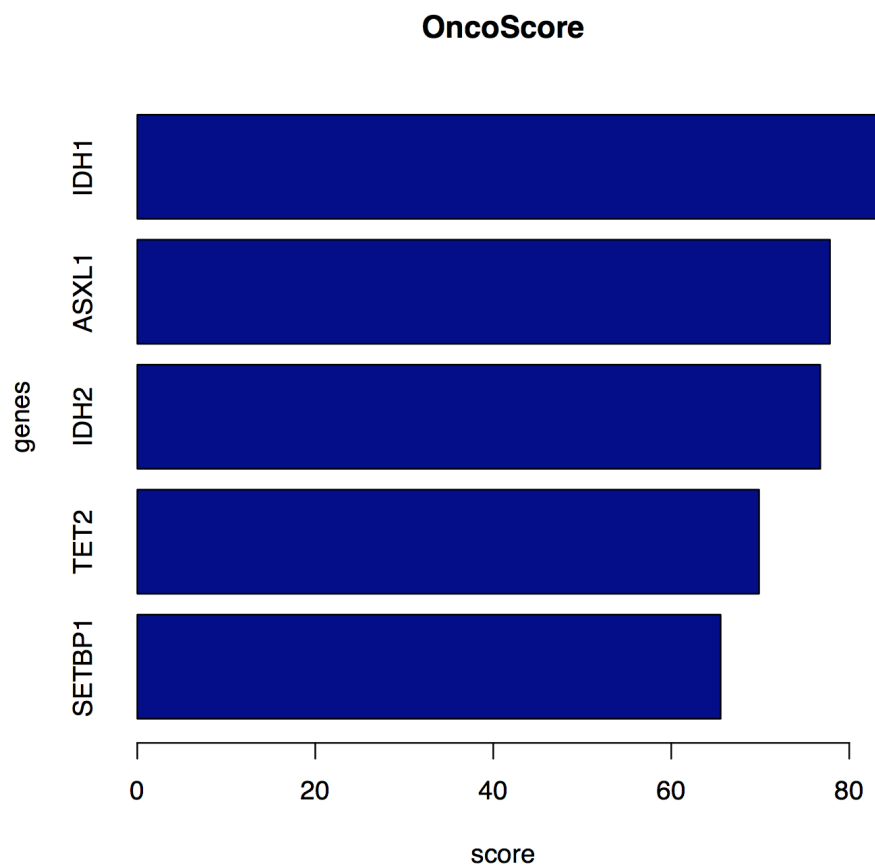

Figure 1: Oncogenetic potential of the considered genes.

```
plot.oncoscore.timeseries(result.timeseries,  
    incremental = TRUE,  
    relative = TRUE,  
    ylab='relative variation')
```

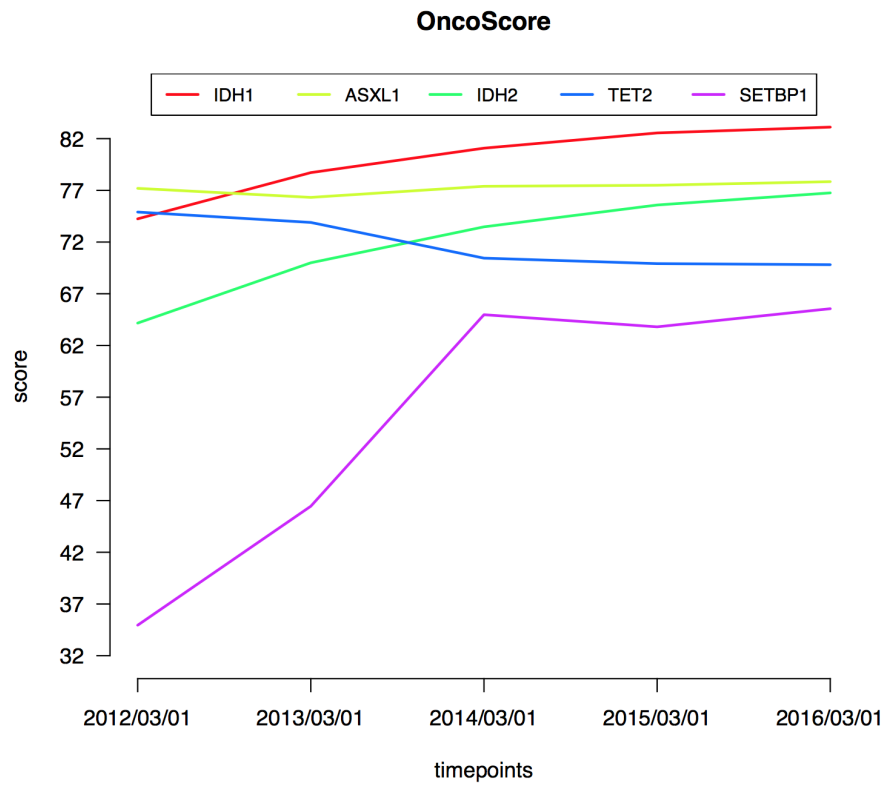

Figure 2: Absolute values of the oncogenetic potential of the considered genes over times.

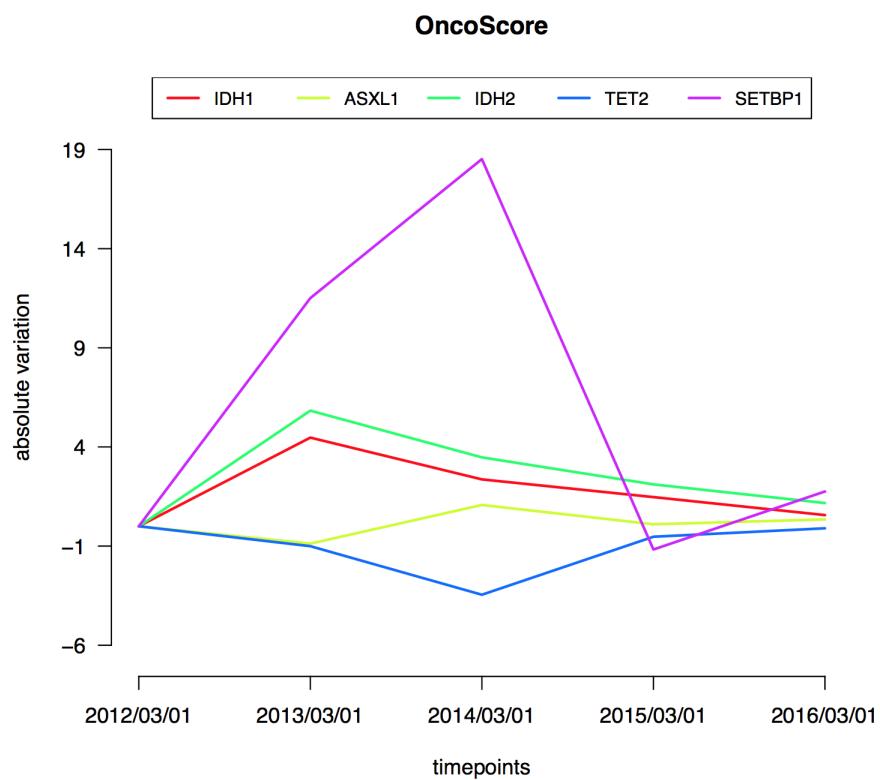

Figure 3: Variations of the oncogenetic potential of the considered genes over times.

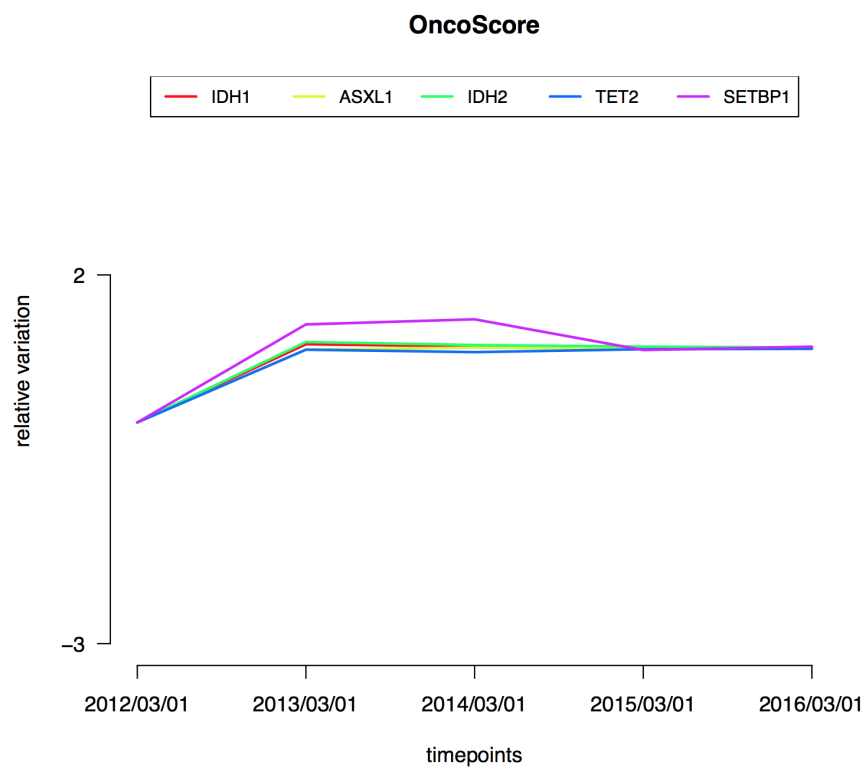

Figure 4: Variations as relative values of the oncogenetic potential of the considered genes over times.
